# Supplementary material for: Sequential Causal Imitation Learning with Unobserved Confounders
Source: arXiv:2208.06276 source file (2022-08-12)
Supplement: Supplementary file 1 [file appendix.tex]

\begin{lemma}
    \label{lemma:markov_boundary_backdoor}
    If there is a set $\bm{Z}\subseteq \before(X_i)$ that satisfies the backdoor criterion for $X_i$, then taking $\mathcal{G}^Y$ as the ancestral graph of $Y$, the Markov Boundary $\bm{Z}'$ of $X_i$ in $\mathcal{G}^Y_{\underline{X_i}}$ also satisfies the backdoor criterion in $\mathcal{G}$
\end{lemma}

\begin{proof}
We know that if $\*Z'$ exists, $(Y\indep X_i |\bm{Z}')$ in $\mathcal{G}^Y_{\underline{X_i}}$ by definition of Markov Boundary.

All we need to show is that if $\*Z\subseteq \before(X_i)$ exists, then $\bm{Z}'\subseteq \before(X_i)$. With outgoing edges from $X_i$ removed in $\mathcal{G}^Y_{\underline{X_i}}$, the boundary simplifies to $\Pa^+(\bm{C}(X_i))\setminus \{X_i\}$, and in the ancestral graph of $Y$, each element of $\bm{C}(X_i)$ is an ancestor of $Y$, and so has an element of $\bm{Z}\subseteq \before(X_i)$ blocking each such path - and
 therefore $\Pa^+(\bm{C}(X_i))\subseteq \before(X_i)$ too.
\end{proof}

\begin{proposition}
    \label{prop:notimitable}
    The distribution of $X_1,X_2$ is not imitable with respect to $Y$ in \Cref{fig:nosequential}.
\end{proposition}

\begin{proof}
    Define the following functional dependence between the nodes in the causal diagram \Cref{fig:nosequential}, where $\oplus$ represents XOR:
    \[
        \begin{aligned}
            U_1 & := \text{Bernoulli}(0.5) \ \ \ \  & \ \ \ \  U_2 & := \text{Bernoulli}(0.5)     \\
            Z   & := U_1 \oplus U_2                 & X_1          & := Z                         \\
            X_2 & := U_2                            & Y            & := ((X_1 \oplus X_2) == U_1) \\
        \end{aligned}
    \]

    The idea above is to encode information about $U_1$ in $X_1,X_2$, which can then be verified by $Y$. In particular,
    \[
        Y=((X_1 \oplus X_2) == U_1) = (( (U_1 \oplus U_2)\oplus U_2) == U_1) = (U_1 == U_1) = 1
    \]

    Notice that the value of $Y$ compares the imitated values $X_1,X_2$ to $U_1$. Without any way to observe $U_1$, the imitator has no way of guessing correctly more than $50\%$ of the time.

    More rigorously, the imitator has a distribution determined by a function $f(Z) \rightarrow (X_1,X_2)$, since only $Z$ is observed. The problem of imitation here can therefore be reduced to finding values for an output distribution for $f$ that result in a distribution over $Y$ identical to the demonstrator's observational distribution:

    The demonstrator's (i.e. natural) distribution is as follows, which has $P(Y=1)=1$
    \begin{center}
        \begin{tabular}{ c c c c c c | c}
            $U_1$ & $U_2$ & $Z$ & $X_1$ & $X_2$ & $Y$ & $P(...)$ \\
            \hline
            0     & 0     & 0   & 0     & 0     & 1   & 0.25     \\
            0     & 1     & 1   & 1     & 1     & 1   & 0.25     \\
            1     & 0     & 1   & 1     & 0     & 1   & 0.25     \\
            1     & 1     & 0   & 0     & 1     & 1   & 0.25     \\
        \end{tabular}
    \end{center}

    The target distribution over the imitating function can be written as a set of variables:
    \begin{center}
        \begin{tabular}{ c | c c  | c}
            $Z$ & $X_1$ & $X_2$ & $P(f(Z)\rightarrow (X_1,X_2)|Z)$ \\
            \hline
            0   & 0     & 0     & $a_0$                            \\
            0   & 0     & 1     & $a_1$                            \\
            0   & 1     & 0     & $a_2$                            \\
            0   & 1     & 1     & $1-a_0-a_1-a_2$                  \\
            \hline
            1   & 0     & 0     & $b_0$                            \\
            1   & 0     & 1     & $b_1$                            \\
            1   & 1     & 0     & $b_2$                            \\
            1   & 1     & 1     & $1-b_0-b_1-b_2$                  \\
        \end{tabular}
    \end{center}

    Using this, we can now compute $P(Y=1|U_1=0,U_2=0)$, where $Z=U_1 \oplus U_2  =0$, giving
    $P(X_1\oplus X_2 = 1) = a_1 + a_2$ - this means that $P(Y=1|U_1=0,U_2=0)=1-a_1-a_2$, meaning that $a_1=0$ and $a_2=0$ to match the demonstrator's distribution (demonstrator never has $Y=0$).

    Next, we compute $P(Y=1|U_1=1,U_2=1)$, with $Z = U_1 \oplus U_2  =0$ once again. $P(X_1\oplus X_2 = 1) = a_1 + a_2$ once again, giving $P(Y=1|U_1=1,U_2=1)=a_1+a_2$, which must add up to $1$ - but we already required that both variables were 0 to satisfy the previous requirement.

    This means that there exists no assignment to the imitator's probabilities that has $P(Y=1)$.
\end{proof}

\begin{figure}
    \begin{subfigure}{0.31\linewidth}
        \centering
        \begin{tikzpicture}
            \node[vertex,dashed,red,thick] (y) at (0,-1) {$Y$};

            \node[vertex,dashed] (u3) at (-1,1) {$U_3$};
            \node[vertex] (z3) at (0,0.5) {$Z_3$};

            \node[vertex,dashed] (u2) at (2,3.7) {$U_2$};
            \node[vertex,blue,thick] (x3) at (0,2) {$X_3$};
            \node[vertex] (z2) at (1,3) {$Z_2$};
            \node[vertex,blue,thick] (x2) at (0,3.5) {$X_2$};
            \node[vertex,dashed] (u1) at (0,5.3) {$U_1$};
            \node[vertex,blue,thick] (x1) at (1,4.5) {$X_1$};
            \node[vertex] (z1) at (-1,4.5) {$Z_1$};

            \path (u3) edge (y);
            \path (z3) edge (y);
            \path (u3) edge (z3);

            \path (u2) edge (z2);
            \path (u2) edge (z3);

            \path (x1) edge (x2);
            \path (x1) edge (u2);
            \path (u1) edge (z1);
            \path (u1) edge (x1);
            \path (u1) edge (z2);
            \path (z1) edge (x2);
            \path (x2) edge (x3);
            \path (x3) edge (z3);
            \path (z2) edge (x3);

        \end{tikzpicture}
        \caption{\label{fig:bdchain}}
    \end{subfigure}
    \begin{subfigure}{0.31\linewidth}
        \centering
        \begin{tikzpicture}
            \node[vertex,dashed,red,thick] (y) at (0,-1) {$Y$};

            \node[vertex,dashed,orange,thick] (u3) at (-1,1) {$U_3$};
            \node[vertex] (z3) at (0,0.5) {$Z_3$};

            \node[vertex,dashed,orange,thick] (u2) at (2,3.7) {$U_2$};
            \node[vertex,blue,thick] (x3) at (0,2) {$X_3$};
            \node[vertex] (z2) at (1,3) {$Z_2$};
            \node[vertex,blue,thick] (x2) at (0,3.5) {$X_2$};
            \node[vertex,dashed,orange,thick] (u1) at (0,5.3) {$U_1$};
            \node[vertex,blue,thick] (x1) at (1,4.5) {$X_1$};
            \node[vertex] (z1) at (-1,4.5) {$Z_1$};

            \path[orange,thick] (u3) edge (y);
            \path (z3) edge (y);
            \path[orange,thick] (u3) edge (z3);

            \path[orange,thick] (u2) edge (z2);
            \path[orange,thick] (u2) edge (z3);

            \path (x1) edge (x2);
            \path (x1) edge (u2);
            \path (u1) edge (z1);
            \path[orange,thick] (u1) edge (x1);
            \path[orange,thick] (u1) edge (z2);
            \path (z1) edge (x2);
            \path (x2) edge (x3);
            \path (x3) edge (z3);
            \path (z2) edge (x3);

        \end{tikzpicture}
        \caption{\label{fig:bdchain_bdpath}}
    \end{subfigure}
    \begin{subfigure}{0.31\linewidth}
        \centering
        \begin{tikzpicture}
            \node[vertex,dashed,red,thick] (y) at (0,-1) {$Y$};

            \node[vertex,dashed,orange,thick] (u3) at (-1,1) {$U_3$};
            \node[vertex] (z3) at (0,0.5) {$Z_3$};

            \node[vertex,dashed,orange,thick] (u2) at (2,3.7) {$U_2$};
            \node[vertex,blue,thick] (x3) at (0,2) {$X_3$};
            \node[vertex] (z2) at (1,3) {$Z_2$};
            \node[vertex,blue,thick] (x2) at (0,3.5) {$X_2$};
            \node[vertex,dashed,orange,thick] (u1) at (0,5.3) {$U_1$};
            \node[vertex,blue,thick] (x1) at (1,4.5) {$X_1$};
            \node[vertex] (z1) at (-1,4.5) {$Z_1$};

            \path[orange,thick] (u3) edge (y);
            \path[line width=.1cm] (z3) edge (y);
            \path[orange,thick] (u3) edge (z3);

            \path[orange,thick] (u2) edge (z2);
            \path[orange,thick] (u2) edge (z3);

            \path[line width=.1cm] (x1) edge (x2);
            \path[gray] (x1) edge (u2);
            \path[gray] (u1) edge (z1);
            \path[orange,thick] (u1) edge (x1);
            \path[orange,thick] (u1) edge (z2);
            \path[gray] (z1) edge (x2);
            \path[line width=.1cm] (x2) edge (x3);
            \path[line width=.1cm] (x3) edge (z3);
            \path[line width=.1cm] (z2) edge (x3);

        \end{tikzpicture}
        \caption{\label{fig:bdchain}}
    \end{subfigure}

    \caption{An example non-imitable query (\Cref{prop:notimitable2}) that is used to demonstrate the ideas of \Cref{thm:nobdchain} is shown in (a). A ``bidirected path'' through the latents is shown in (b), and the XOR tree constructed from the path is in (c).}
\end{figure}

\begin{proposition}
    \label{prop:notimitable2}
    The distribution of $X_1,X_2,X_3$ is not imitable with respect to $Y$ in \Cref{fig:bdchain}.
\end{proposition}

\begin{proof}
    This example is used as a demonstration of the ideas behind the proof of \Cref{thm:nobdchain}. We notice that there is a latent chain $Y\leftarrow U_3 \rightarrow Z_3 \leftarrow U_2 \rightarrow Z_2 \leftarrow U_1 \rightarrow X_1$ (\Cref{fig:bdchain_bdpath}), which shows that $Y$ and $X_1$ are in the same ancestral c-component.

    We will construct an equation of XORs made up of the values of the latent variables in the above chain, such that each latent variable except $U_3$ is used twice, canceling itself, so that $Y$ can check if the chain correctly cancelled with a comparison to $U_3$.

    To witness, we have:
    \[
        \begin{aligned}
            U_1,U_2,U_3 & \sim Bernoulli(0.5)                                                         \\\\
            Z_1         & = 1                                                                         \\
            X_1         & = U_1                                                                       \\
            X_2         & = X_1                                                                       \\
            Z_2         & = U_1 \oplus U_2                                                            \\
            X_3         & = X_2 \oplus Z_2            & \Rightarrow & U_1 \oplus U_1 \oplus U_2 = U_2 \\
            Z_3         & = X_3 \oplus U_2 \oplus U_3 & \Rightarrow & U_2 \oplus U_2 \oplus U_3 = U_3 \\
            Y           & = (Z_3==U_3)                & \Rightarrow & (U_3==U_3) = 1
        \end{aligned}
    \]

    Critically, we can now show that without a way to observe $X_1$ or $U_1$, it is now impossible to correctly set the values incoming to $Y$:

    \[
        Y = (Z_3==U_3) =  ((X_3 \oplus U_2 \oplus U_3) == U_3) = ((f(Z_1,Z_2) \oplus U_2 \oplus U_3) == U_3)
    \]

    Since $X_3$ is imitated, it must be a function of the observed variables ($X_1,X_2$ are generated, the imitator does not observe what they would have been had the imitator not performed any action).

    The only way to satisfy the above equation is $f(Z_1,Z_2) == U_2$. However, we can substitute: $f(Z_1,Z_2) = f(1,U_1 \oplus U_2)$. With no additional knowledge, there is no way to disentangle $U_1 \oplus U_2$, meaning that there does not exist a function $f$ that outputs $U_2$ from the given inputs.
\end{proof}

\begin{restatable}{theorem}{nobdchain}
    \label{thm:nobdchain}
    Let $\mathcal{G}^Y$ be the ancestral graph of $Y$ in $\mathcal{G}$. If there is $X_i\in \bm{X}$ such that $X_i\in \bm{C}(Y)$, then $\bm{X}$ is not imitable with respect to $Y$ in $\mathcal{G}$.
\end{restatable}

\begin{proof}
    An example of the steps taken in this proof is given in \Cref{prop:notimitable2}. Let the corresponding chain of latent variables be $Y \leftarrow U_1 \rightarrow V_1 \leftarrow U_2 \rightarrow ... \leftarrow U_n \rightarrow X_i$. WLOG, we can assume that the chain does not repeat nodes (if it did, then it has a cycle, and we can create another chain with the cycle removed), and that none of the $V_j$ are imitated (we can shorten the chain to the first element of $X$ along it).

    We construct a model for the given graph as follows:
    \begin{itemize}
        \item Create a tree $T$ rooted at $Y$ which will hold the scaffolding for our constructed distribution. Since this is an ancestral graph, each node has a directed path to $Y$. For each $V_1,...V_{n-1},X_i$ in reverse topological order, find a single directed path from the node to either $Y$ or a node along a previously found path, whichever intersects first. Define the set of nodes along these paths (including $V$ and $X_i$) as $P$.
        \item Each of $V_1,...V_{n-1}$ has 2 inputs from the chain (as well as possibly other inputs). Let the value $V_i = U_i \oplus U_{i+1} \bigoplus_{P_j\in (Pa(V_i)\cap P)} P_j$.
        \item Each element $P\setminus V$ is defined as $P_i = \bigoplus_{P_j\in (Pa(P_i)\cap P)} P_j$
        \item $X_i = U_n \bigoplus_{P_j\in (Pa(X_i)\cap P)} P_j$
        \item $Y = (U_1 == \bigoplus_{P_j\in (Pa(Y)\cap P)} P_j)$
        \item Let all $U_i \sim Bernoulli(0.5)$
        \item All other variables are set to $1$
    \end{itemize}

    The model's construction is consistent with the causal graph, and results in $Y=1$ with probability 1.

    We now show that the imitator has no way of reconstructing $Y=1$. Define $T'$ as the subtree of $T$ which, starting at $Y$, stops at the first element of $X$, or at the end of the path in $P$. Let these sub-paths be $P'$. The equation resulting for the imitated $Y$ is therefore:
    \[
        Y= \left(U_1 == \left(\bigoplus_{V_i \in V\cap T'} (U_i \oplus U_{i+1}) \right) \left(\bigoplus_{X_i \in X\cap T'} X_i\right) \right)
    \]

    We now imagine a \textit{stronger} version of the imitator, which replaces the possibly multiple $\bigoplus_{X_i \in X\cap T'} X_i$ with a single function $f$, which has as inputs \textit{all possible observed information}, including information computed \textit{after} the action $X$ is taken.

    To achieve this, we observe that only the $V_i$ have values not completely determined by their observed parents. We define $V_i' = U_i \oplus U_{i+1} $, which can be computed from the observed values by xoring with its parents. This means the $V_i'$ contain all of the information from the observed values - and are well-defined even for future nodes (nodes that depend on an imitation decision).

    This means that the function $f$ has more information than the actual imitator. We will show that even this weaker version of the problem is not imitable:
    \[
        Y= \left(U_1 == \left(\bigoplus_{V_i \in V\cap T'} (U_i \oplus U_{i+1}) \right) \oplus f(V'_1,...,V'_{n-1}) \right)
    \]

    Since $V'_i= U_i \oplus U_{i+1}$, we can redefine $f' =\bigoplus_{V_i \in V\cap T'} (V_i')  \oplus f$ to reduce the above equation to:
    \[
        Y= \left(U_1 ==  f'(U_1\oplus U_2,...,U_{n-1}\oplus U_{n}) \right)
    \]

    $U_1$ is only present in $V'_1$, so it must be used in $f$, but then $U_2$ must be isolated to extract the value of $U_1$. This proceeds recursively along the chain until $U_n$ is reached, which is not present in any other observed variable, allowing us to conclude that it is not possible to isolate $U_1$ in $f'$.

    This shows that even a generalized imitator that has access to future information cannot perform imitation here, and so the above distribution is not imitable.
\end{proof}

\begin{restatable}{theorem}{recursivemfactor}
    \label{thm:recursivemfactor}
    Suppose that there exists an m-factor $(\bm{V}^X,\bm{X},\bm{Z},Y)$ in $\mathcal{G}$, and let $\bm{X}'=\{X_2,...,X_n\}$ ($\bm{X}$ with the first element in temporal order removed). Then there exists sets $\bm{V}^{X'},\bm{Z}'$ such that $(\bm{V}^{X'},\bm{X}',\bm{Z}',Y)$ is an m-factor for $\mathcal{G}$.
\end{restatable}
%\recursivemfactor*

\begin{proof}
    Let $X_1$ be the removed variable. Note that since $X_1$ comes first in temporal order, none of its ancestors are in $\bm{X}$. There are two cases of interest.

    The first is when $X_1 \not\in \bm{X}^B$. In this case, the new m-factor is simply $(\bm{V}^X,\bm{X}',\bm{Z},Y)$. Since the conditioning sets and $\bm{V}^Y$ remain identical, the m-factor conditions hold directly for the new set.

    In the case where $X_1\in \bm{X}^B$, we cannot directly remove $X_1$, since there can be elements of $\bm{V}^X$ that are ancestors of $X_1$. We instead show that we can create a new set $\bm{V}^{X'}$ and $\bm{Z}'$ which removes ancestors of $X_1$ from $\bm{V}^X$. In particular, we can instead set $\bm{Z}'=\bm{Z}\cup (\bm{V}^X \cap An(X_1)_{\mathcal{G}_{\underline{\bm{X}^B}}})$, and $\bm{V}^{X'} = \bm{V}^{X}\setminus An(X_1)_{\mathcal{G}_{\underline{\bm{X}^B}}}$. We show that the resulting set satisfies the requirements of an m-factor.
    \begin{enumerate}
        \item Since $An(X_1)_{\mathcal{G}_{\underline{\bm{X}^B}}}$ were the only elements removed from $\bm{V}^X$ and added to $\bm{V}^Y$, we know that $\bm{X}'\in \bm{V}^{X'}$, since $X_1$ was the first element of $\bm{X}$ in temporal order (so none of its ancestors are in $\bm{X}'$). Likewise, $Z'\subseteq \bm{V}^Y$, since $\bm{V}^{Y'}=\bm{V}^{Y} \cup An(X_1)_{\mathcal{G}_{\underline{\bm{X}^B}}}$, which inludes $\bm{Z}\subseteq \bm{V}^Y$ and $(\bm{V}^X \cap An(X_1)_{\mathcal{G}_{\underline{\bm{X}^B}}}) \subseteq An(X_1)_{\mathcal{G}_{\underline{\bm{X}^B}}}$.
        \item Since all ancestors of $X_1$ in $\mathcal{G}_{\underline{\bm{X}^B}}$ are removed from $\bm{V}^{X'}$, any element in $\bm{X}^{X'}$ has the same descendants in $\mathcal{G}_{\underline{\bm{X}^B}}$ as the original m-factor.
        \item Suppose not. That is, $\exists V_x\in \bm{V}^{X'}$ and $V_y\in \bm{V}^{Y'}$ such that $(V_x \not\indep V_y|\bm{Z}')$ in $\mathcal{G}_{\underline{\bm{X}^B}}$. We know that $V_y \notin \bm{V}^X \cap An(X_1)_{\mathcal{G}_{\underline{\bm{X}^B}}}$, because those elements are part of $\bm{Z}'$, and all elements are independent of $V_y$ conditioned on $V_y$. We therefore know that $V_y \in \bm{V}^Y$. Likewise, since $\bm{V}^{X'}\subseteq \bm{V}^{X}$, $V_x \in \bm{V}^{X'}$.
              Suppose that the path crosses colliders $Z_1,Z_2,...,Z_k \in \bm{Z}'$. Suppose that all colliders are from the set $\bm{Z}$, and there are none from $\bm{Z}'\setminus \bm{Z}$. This path also exists in the original m-factor, so we have created an unblocked path which violates condition 2 of the original m-factor, $(\bm{V}^X \indep \bm{V}^Y | \bm{Z})$ - a contradiction. Next, suppose that the colliders can be elements of $\bm{Z}'\setminus \bm{Z}$ (i.e. elements added for the new m-factor). Let $Z_j$ be the last such element along the path. This means that $Z_j \in \bm{V}^X \cap An(X_1)_{\mathcal{G}_{\underline{\bm{X}^B}}}$. Taking only the portion of the path from $Z_j$ to $V_y$, the remaining colliders are from $\bm{Z}$, we have created an unblocked path from $Z_j \in \bm{V}^X$ to $V_y\in \bm{V}^Y$. However, this path cannot exist, since $(\bm{V}^X \indep \bm{V}^Y | \bm{Z})$ by condition 2 of the original m-factor.
        \item Suppose not. That is, suppose that there is an unblocked path in $\mathcal{G}_{\underline{\bm{X}^B}}$ from $X_j\in \bm{X}'$ to $\bm{V}^{Y'}$ conditioned on $(\bm{X}'\cup\bm{Z}')\cap\before(X_j)$. Let $Z_1,...,Z_k$ be the colliders along this path. For each such collider $Z_i$ in $\bm{Z}'\setminus \bm{Z}$, we know that it is an ancestor of $X_1$, and that it has a directed path to it in $\bm{V}^X$. Since $X_1 \in \bm{X}\cap\before(X_j)$ ($X_1$ is first element of $\bm{X}$ in temporal order), we can replace each $Z_i$ collider in the original path with the directed path from $Z_i$ to $X_1$, and the path repeated back to $Z_i$, effectively replacing the collider at $Z_i$ with a collider at $X_1$, creating a path from $X_i$ to $V_y$ conditioned on $(\bm{X}\cup\bm{Z})\cap\before(X_j)$, violating condition 4 of the original m-factor.
    \end{enumerate}
    This completes the conditions, showing that the smaller m-factor always exists when removing the first element of $\bm{X}$ in temporal order from the set of actions.
\end{proof}

\begin{figure}
    \begin{subfigure}{0.24\textwidth}
        \centering
        \begin{tikzpicture}
            \node[vertex]  (a) at (-1,2) {$A$};
            \node[vertex,blue,thick] (x1) at (0,3) {$X_1$};
            \node[vertex] (b) at (0,2) {$B$};
            \node[vertex,blue,thick] (x2) at (0,1) {$X_2$};
            \node[vertex,blue,thick] (x3) at (1,0.1) {$X_3$};
            \node[vertex] (c) at (2,0.5) {$C$};
            \node[vertex,dashed,red,thick] (y) at (0.5,-1) {$Y$};

            \path[bidirected] (x1) edge[bend right=40] (a);
            \path[bidirected] (x3) edge[bend right=40] (x2);
            \path[bidirected] (x3) edge[bend left=40] (c);
            \path (x1) edge (b);
            \path (b) edge (x2);
            \path (x2) edge (y);
            \path (x3) edge (y);
            \path (c) edge (y);
            \path (a) edge (y);

        \end{tikzpicture}
        \caption{\label{fig:imitable_example}}
    \end{subfigure}
    \begin{subfigure}{0.24\textwidth}
        \centering
        \begin{tikzpicture}
            \node[vertex]  (a) at (-1,2) {$A$};
            \node[vertex,blue,thick] (x1) at (0,3) {$X_1$};
            \node[vertex] (b) at (0,2) {$B$};
            \node[vertex,blue,thick] (x2) at (0,1) {$X_2$};
            \node[vertex,orange,thick] (x3) at (1,0.1) {$X_3$};
            \node[vertex] (c) at (2,0.5) {$C$};
            \node[vertex,dashed,red,thick] (y) at (0.5,-1) {$Y$};

            \path[bidirected] (x1) edge[bend right=40] (a);
            \path (x2) edge (x3);
            \path (c) edge (x3);
            \path (x1) edge (b);
            \path (b) edge (x2);
            \path (x2) edge (y);
            \path (x3) edge (y);
            \path (c) edge (y);
            \path (a) edge (y);

        \end{tikzpicture}
        \caption{\label{fig:imitable_example_x1}}
    \end{subfigure}
    \begin{subfigure}{0.24\textwidth}
        \centering
        \begin{tikzpicture}
            \node[vertex]  (a) at (-1,2) {$A$};
            \node[vertex,blue,thick] (x1) at (0,3) {$X_1$};
            \node[vertex] (b) at (0,2) {$B$};
            \node[vertex,orange,thick] (x2) at (0,1) {$X_2$};
            \node[vertex,orange,thick] (x3) at (1,0.1) {$X_3$};
            \node[vertex] (c) at (2,0.5) {$C$};
            \node[vertex,dashed,red,thick] (y) at (0.5,-1) {$Y$};

            \path[bidirected] (x1) edge[bend right=40] (a);
            \path (x2) edge (x3);
            \path (c) edge (x3);
            \path (x1) edge (b);
            \path (a) edge (x2);
            \path (x2) edge (y);
            \path (x3) edge (y);
            \path (c) edge (y);
            \path (a) edge (y);

        \end{tikzpicture}

        \caption{\label{fig:imitable_example_x2}}
    \end{subfigure}
    \begin{subfigure}{0.24\textwidth}
        \centering
        \begin{tikzpicture}
            \node[vertex]  (a) at (-1,2) {$A$};
            \node[vertex,orange,thick] (x1) at (0,3) {$X_1$};
            \node[vertex] (b) at (0,2) {$B$};
            \node[vertex,orange,thick] (x2) at (0,1) {$X_2$};
            \node[vertex,orange,thick] (x3) at (1,0.1) {$X_3$};
            \node[vertex] (c) at (2,0.5) {$C$};
            \node[vertex,dashed,red,thick] (y) at (0.5,-1) {$Y$};

            \path (x2) edge (x3);
            \path (c) edge (x3);
            \path (x1) edge (b);
            \path (a) edge (x2);
            \path (x2) edge (y);
            \path (x3) edge (y);
            \path (c) edge (y);
            \path (a) edge (y);

        \end{tikzpicture}
        \caption{\label{fig:imitable_example_x3}}
    \end{subfigure}
    \caption{An example graph used to demonstrate the procedure used to check a sequential $\pi$-backdoor from \Cref{proposition:imitable}. The temporal observation order of the nodes is: $X_1,A,B,X_2,C,X_3$. This means, for example, that the imitator for $X_2$ has no knowledge of $C$ nor the decision that will be made at $X_3$.}
\end{figure}

\begin{proposition}
    \label{proposition:imitable}
    The distribution shown in figure \Cref{fig:imitable_example} with temporal order $X_1,A,B,X_2,C,X_3$ is imitable using the functions: $X_1 =P(X_1),X_2=P(X_2|A),X_3=P(X_3|X_2,C)$.
\end{proposition}

\begin{proof}

    In the graph shown in \Cref{fig:imitable_example}, we can follow the conditions of \Cref{def:seq_pi_backdoor} iteratively:
    \begin{enumerate}
        \item In \Cref{fig:imitable_example}, which is equivalent to $\1G_3$, since there are no later actions $(X_3\indep Y|X_2,C)_{\underline{X_3}}$, satisfying condition (1).
        \item Once $X_3$ is replaced with the imitating function, we get $\1G_2$, shown in \Cref{fig:imitable_example_x1}. Here, $(X_2\indep Y|A)_{\underline{X_2}}$, once again satisfying condition (1).
        \item Finally, we get $\1G_1$, in \Cref{fig:imitable_example_x2}. While there is no way to condition on $A$ because it comes after $X_1$, $X_1$ is no longer an ancestor of $Y$, so it satisfies condition (2).
    \end{enumerate}
    
    This leads to a final imitating policy shown in \Cref{fig:imitable_example_x3}.
    
    To verify this result, we can now decompose the probability of $Y$ using the independence relations from the given graph:
    \[
        \begin{aligned}
            P(Y) & =  \sum_{A,X_2,X_3,C}P(Y,A,X_2,X_3,C) = \sum_{A,X_2,X_3,C}P(Y|A,X_2,X_3,C)P(A,X_2,X_3,C) \\
                 & = \sum_{A,X_2,X_3,C}P(Y|A,X_2,X_3,C)P(A)P(C)P(X_2|A)P(X_3|AX_2C)
        \end{aligned}
    \]

    When replacing the mechanisms of $X$ with their imitated counterparts, we get the following probability for $Y$:
    \[
        \begin{aligned}
            \hat P(Y) & = \sum_{V\setminus\{Y\}} P(V...,Y) = \sum_{V\setminus\{Y\}}\sum_U P(V...,Y,U...)        \\
            = \sum    & P(Y|AX_2X_3C)P(A|U_1)P(U_1)P(X_1)P(B|X_1)P(X_2|A)P(U_2)P(X_3|CX_2A)P(U_3)P(C|U_3)P(U_3) \\
                      & = \sum_{V\setminus\{Y\}}  P(Y|AX_2X_3C)P(A)P(B,X_1)P(X_2|A)P(X_3|CX_2A)P(C)             \\
                      & = \sum_{A,X_2,x_3,C} P(Y|AX_2X_3C)P(A)P(X_2|A)P(X_3|CX_2A)P(C)                          \\
        \end{aligned}
    \]

    These equations match, showing that the given mechanisms are sufficient for imitation.
\end{proof}
